# Supplementary material for: SecretBench: A Dataset of Software Secrets
Source: arXiv:2303.06729 source file (2023-03-12)
Supplement: Supplementary file 1 [file Appendix.tex]

\input{Tables/QuestionCountPerYear}
\input{Tables/tagskeywords}
\input{Tables/FinalAnswerMappingsTables}
